# Supplementary material for: Organize, Then Vote: Exploring Cognitive Load in Quadratic Survey Interfaces
Source: arXiv:2503.04114 source file (2025-05-16)
Supplement: Supplementary file 1 [file interface_exisiting.tex]

\newpage
\section{Other Existing QV Interfaces}
\label{apdx:otherQV}
In this section, we list out other QV interfaces we surveyed.

\begin{figure}[h!]
    \centering
    \includegraphics[width=0.6\textwidth]{content/image/curr_interface/cheng_qv.png}
    \caption{The interface used in the research by~\textcite{chengCanShowWhat2021}.}
    \label{fig:raymondQV}
\end{figure}

\begin{figure}[h!]
    \centering
    \includegraphics[width=0.6\textwidth]{content/image/curr_interface/geek.sg_interface.png}
    \caption{An open-source QV interface~\cite{yehjxraymondYehjxraymondQvapp2024} that offers a publicly available service.}
    \label{fig:raymondQV}
\end{figure}

\begin{figure}[h!]
    \centering
    \includegraphics[width=0.6\textwidth]{content/image/curr_interface/appvote.png}
    \caption{The interface designed for gov4git~\cite{Gov4gitDecentralizedPlatform2023}.}
    \label{fig:gov4gitQV}
\end{figure}

\newpage
% \begin{figure}
%     \centering
%     \includegraphics[width=0.6\textwidth]{content/image/curr_interface/QVSR.png}
%     \caption{The interface used within recent preprint for QV for survey research by~\textcite{cavaille2024cares}}
%     \label{fig:qvsr}
% \end{figure}
